# Supplementary material for: Dynamics-Aware Quality-Diversity for Efficient Learning of Skill Repertoires
Source: arXiv:2109.08522 source file (2021-09-16)
Supplement: Supplementary file 1 [file appendix.tex]

\section*{Appendix}
\section{Pseudo-code} \label{appendix:pseudo-code}
The pseudo-code for Dynamics-Aware Quality-Diversity is provided in Algorithm~\ref{algo:mb-qd}. 

\algnewcommand{\LeftComment}[1]{\State \(\triangleright\) #1}

\begin{algorithm}[ht!]
  \small
% \SetAlgoLined
% \DontPrintSemicolon

\caption{\algonamefull{} (\algoname{})}
  
\label{algo:mb-qd}
  \begin{algorithmic}[1]

 \State{Initialize repertoire $\archivereal$ (to $\varnothing)$, imagined repertoire $\archivesynthetic$ (to $\varnothing$), dynamics model $\dynamicsmodel$, and replay buffer $\replaybuffer$ (to $\varnothing)$}
 \\
 \While{maximum number of evaluations not reached}
 \\
  \If{first iteration} \Comment{\textit{Generate random policies at first iteration.}}
      \State{$\batchpoliciesrealmutated \leftarrow$ random\_parameters()}

  \Else
        \State{$\batchpoliciesreal \leftarrow$ select($\archivereal$) \Comment{\textit{Selecting $b$ policies from repertoire $\archivereal$ (section~\ref{sec:background}).}}}
        \State{$\batchpoliciesrealmutated \leftarrow$ variation\_operators($\batchpoliciesreal$) \Comment{\textit{Apply variations to parameters $\param{i}$.}}}
    \EndIf
    \\
    
    \LeftComment{\textit{Performing QD Exploration in Imagination (section~\ref{sec:methods-qd_exploration_imag})}}
  \While{model stopping criterion is False}
  
    \State{$(\widetilde{\skilldescriptor_i}, \widetilde{\reward_i})_{i\in\left[1,b\right]} \leftarrow$ imagined\_rollouts($\batchpoliciesrealmutated$) using $\dynamicsmodel$ \Comment{\textit{Evaluate using dynamics model. }}}
    
    \State{$\archivesynthetic$ $\leftarrow$ model\_condition($\batchpoliciesrealmutated,\archivesynthetic$) \Comment{\textit{Add $\policyrealmutated{i}$ to $\archivesynthetic$ depending on $\widetilde{\reward_i}$ and novelty of $\widetilde{\skilldescriptor_i}$.}}}
    
    \If{model stopping criterion is False} \Comment{\textit{Continue performing QD exploration in imagination.}}
    
        \State{$\batchpoliciesreal \leftarrow$ select($\archivesynthetic$) \Comment{\textit{Selecting $b$ policies from imaginary repertoire $\archivesynthetic$.}}}
        
        \State{$\batchpoliciesrealmutated \leftarrow$ variation\_operators($\batchpoliciesreal$)}
        
    \EndIf
  \EndWhile
  
\\
\LeftComment{\textit{Acting in the Environment (section~\ref{sec:methods-acting_in_env})}}
  \State{$\batchpoliciesreal[N]{}$ $\leftarrow$ select($\archivesynthetic$) \Comment{\textit{Selecting $N$ policies from imaginary repertoire $\archivesynthetic$ to be evaluated.}}}
  
  \State{($\skilldescriptor_i, \reward_i)_{i\in\left[1,N\right]}$, transitions $\leftarrow$ evaluation($\batchpoliciesreal[N]{}$) \Comment{\textit{Evaluate in environment; get transitions.}}}
  \State{$\replaybuffer \leftarrow$ add\_to\_replay\_buffer(transitions, $\replaybuffer$)}
  
  \State{$\archivereal$ $\leftarrow$ repertoire\_condition($\batchpoliciesreal[N]{}, \archivereal$) \Comment{\textit{Add $\policyreal{i}$ to $\archivereal$ depending on $\reward_i$ and novelty of $\skilldescriptor_i$.}}}
  
  \State{$\archivesynthetic$ $\leftarrow$ synchronise\_repertoires($\archivereal$, $\archivesynthetic$)
  \Comment{\textit{Erase content of $\archivesynthetic$ and replace it with the content from $\archivereal$.}}}

  \\
  \LeftComment{\textit{Learning Dynamics Models (section~\ref{sec:methods-dyn_model})}}
  \State{Update $\dynamicsmodel$ using $\replaybuffer$ \Comment{\textit{Train dynamics model with transitions collected in replay buffer.}}}
  
  \EndWhile
  \\
  \State \Return $\archivereal$
  \end{algorithmic}
\end{algorithm}

\section{Implementation Details}
Our QD implementation builds on pymap\_elites~\cite{vassiliades2016using, mouret2020quality} and extends it for our use case. We conducted all simulation experiments with the Dynamic Animation and Robotics Toolkit (DART) simulator~\cite{lee2018dart}.

\subsection{Addition Condition for Unstructured Containers} \label{appendix:addition}
This section provides additional details regarding the unstructured container~\cite{cully2017quality}, that is  explained in section~\ref{sec:background}. 

% After computing the novelty score and return of the policies and considering the two addition conditions (detailed in \ref{sec:background}), a parameter $\epsilon$ is also considered in the addition condition. $\epsilon$ allows more flexibility in the overall addition condition for policies that could potentially improve the entire repertoire to be added even though not immediately satisfying the main two conditions. See~\cite{cully2017quality} for a detailed explanation and experimentation of this.

\newcommand{\pinew}{\pi_{new}}

Before attempting to add a policy $\pinew$ to an unstructured repertoire, we evaluate its return $\reward_{\pinew}$, its skill descriptor $\skilldescriptor_{\pinew}$, and novelty score $nov_{\pinew}$ (see equation~\ref{equation:novelty-score}).
We also find the two nearest neighbors of $\pi$ present in the repertoire (the distance between policies corresponds to the euclidian distance between their respective skill descriptors).
In the following, the first and second nearest neighbors of $\pinew$ from the repertoire are respectively denoted $\pi_1$ and $\pi_2$

If the distance of $\skilldescriptor_{\pinew}$ to its nearest neighbor from the repertoire $\skilldescriptor_{\pi_1}$ is higher than a pre-defined threshold $l$, then $\pinew$ is added to the unstructured repertoire.

Otherwise, $\pinew$ may still replace its nearest neighbor $\pi_1$ in the repertoire if the following conditions are satisfied:
\begin{align}
\label{eq:cond_1}
    \|\skilldescriptor_{\pinew} - \skilldescriptor_{\pi_2}\|_2 &\geqslant l \\
    \label{eq:cond_2}
    nov_{\pinew} &\geqslant (1-\epsilon) nov_{\pi_1} \\
    \label{eq:cond_3}
    \reward_{\pinew} &\geqslant (1 - \epsilon)\reward_{\pi_1} \\ 
    \label{eq:cond_4}
    \left(nov_{\pinew} - nov_{\pi_1}\right)
    |\reward_{\pi_1}| &\geqslant 
    -\left( \reward_{\pinew} - \reward_{\pi_1} \right) |nov_{\pi_1}|
\end{align}
where $\epsilon$ is a parameter in $\left[0, 1\right)$. Condition~\ref{eq:cond_1} ensures that $\pinew$ is novel enough compared to the container policies except $\pi_1$.
Conditions~\ref{eq:cond_2} to~\ref{eq:cond_4} ensure that $\pinew$ outperforms $\pi_1$ with respect to the novelty or the return.
In particular, conditions~\ref{eq:cond_2} and~\ref{eq:cond_3} are there to prevent $\pinew$ from being significantly outperformed by $\pi_1$.
When $\epsilon$ increases, those replacement conditions become more flexible.
See~\cite{cully2017quality} for a detailed explanation and experimentation of this mechanism.

\subsection{Quality-Diversity Exploration}
The hyperparameters used for QD skill discovery of the repertoires are as follows:
\begin{itemize}[noitemsep, leftmargin=8mm]
    \item For the repertoire addition condition, the distance threshold $l$ is set to $0.015$, $\epsilon = 0.1$ and $k = 15$ (see sections~\ref{sec:background} and~\ref{appendix:addition}).
    \item $\sigma_1 = 0.01$ and $\sigma_2 = 0.2$ for directional variation (see equation~\ref{equation:directional-variation}).
\end{itemize} 
We use 32 CPU cores per replication of the skill discovery. As mentioned in the caption of Figure~\ref{fig:hexa_omni_ablation}, we stop the execution of the algorithm as soon as less than one policy is added to the imagined repertoire in one iteration. As the algorithm approaches convergence (i.e. when the skill space gets fully explored), the number of skills that are added to the imagined repertoire significantly decreases. 
Since we only evaluate solutions that have been added to the imagined repertoire, the number of evaluated solutions decreases as we approach convergence.
This results in a total number of evaluations that is lower than the other approaches (Fig.~\ref{fig:hexa_omni_ablation}).
%
%Consequently, the stopping criterion for the QD exploration in imagination requires more imagined rollouts to be reached; and evaluations happen less frequently.
%

%As a consequence, we stop \algoname{} as soon as less than one skill is added to the imagined archive.
% IMPORTANT TODO
%Technical details about the model running to the end and stopping after a certain number of evaluations

\subsection{Dynamics Model}
The dynamics model $\dynamicsmodel$ consists of an ensemble of four probabilistic neural networks.
Each of these neural networks takes as input the current state $\vec s_t$ and action $\vec a_t$ and outputs a normal distribution over the next state $\vec s_{t+1}$.
The state $\vec s_t$ consists of the following: 
\begin{itemize}[noitemsep, leftmargin=8mm]
    \item linear and angular positions and velocities of the torso (center of mass).
    \item all joint angles and velocities.
\end{itemize}
In total, the state has $12+36=48$ dimensions.
The action $\vec a_t$ corresponds to the 18 desired joint angles. 
Each probabilistic neural network outputs the parameters of a normal distribution for the next state $\vec s_{t+1}$.
More specifically, the dynamics model outputs the mean $\vec\mu = \left( \mu_1, \cdots, \mu_{48} \right)$ and a vector of logarithms of standard deviations $\left(\log \sigma_1, \cdots, \log \sigma_{48}\right)$ (the covariance matrix of the normal distribution is considered diagonal).

Each probabilistic neural network is a Multi-Layer Perceptron with two hidden layers of size 500 with ReLU activation functions.
The dynamics model is trained using the Adam optimizer with a learning rate of $10^{-3}$, $\beta_1=0.9$, $\beta_2=0.999$ and a batch size of $512$.
It is trained every 500 evaluations with the transitions present in the replay buffer.
The size of the replay buffer is $10^6$ transitions.

% The hyperparameters related to the architecture and the training of the dynamics model and replay buffer are as follows:
% \begin{itemize}[noitemsep, leftmargin=8mm]
% \vspace{-1mm}
%     \item Replay buffer size of $10^6$.
%     \item Dynamics model with two hidden layers of size 500 with ReLU activations.
%     \item Dynamics model is trained with a learning rate of $10^{-3}$ and batch size of 512, with the Adam optimizer.
%     \item Dynamics model is trained every 500 evaluations.
% \end{itemize}
%States used for the dynamics model consists of the linear and angular positions and velocities of the torso (CoM) of the robot and the joint positions velocities of the robot. The action space used for the dynamics model consists of the 18 desired joint angles.

\subsection{Hexapod Robot Platform}
As mentioned in Section \ref{sec:exps-envs}, we use an 18 DoF hexapod robot that is open-sourced. The robot consists of Dynamixel XM430-W350-R motors. Link to the robot design and setup will be available once the review process is complete.

\section{Additional Experimental Details}
\subsection{Hexapod Omni-directional Skill}
The skill space referred to in Section \ref{sec:exps-sample_eff} has $\skilldescriptor$ defined as the following:
\begin{equation*}
    \skilldescriptor = 
    \begin{pmatrix}
    x_T  \\
    y_T  \\ 
    \end{pmatrix}
\end{equation*}
where $x_T$ and $y_T$ are the relative cartesian displacements of the robot at the end of the episode $T$. The return $\reward$ is defined as:
\begin{equation*}
    \reward = |\alpha_i-\alpha_d|
\end{equation*}
where $\alpha_i$ is the relative yaw angle of the robot at the end of the episode $T$ and $\alpha_d$ is the desired angle defined by a circular trajectory. Figure~\ref{fig:hexa_omni_ablation}A illustrates this. 

Defining the $\skilldescriptor$ in this way allows skill policies that result in diversity in the $\left(x,y\right)$ space to be discovered. Figure \ref{fig:omni-rep-viz} shows the repertoire of skills discovered and three sampled example trajectories of executed skills. 
\begin{figure}[h]
\centering
	\includegraphics[width=\linewidth]{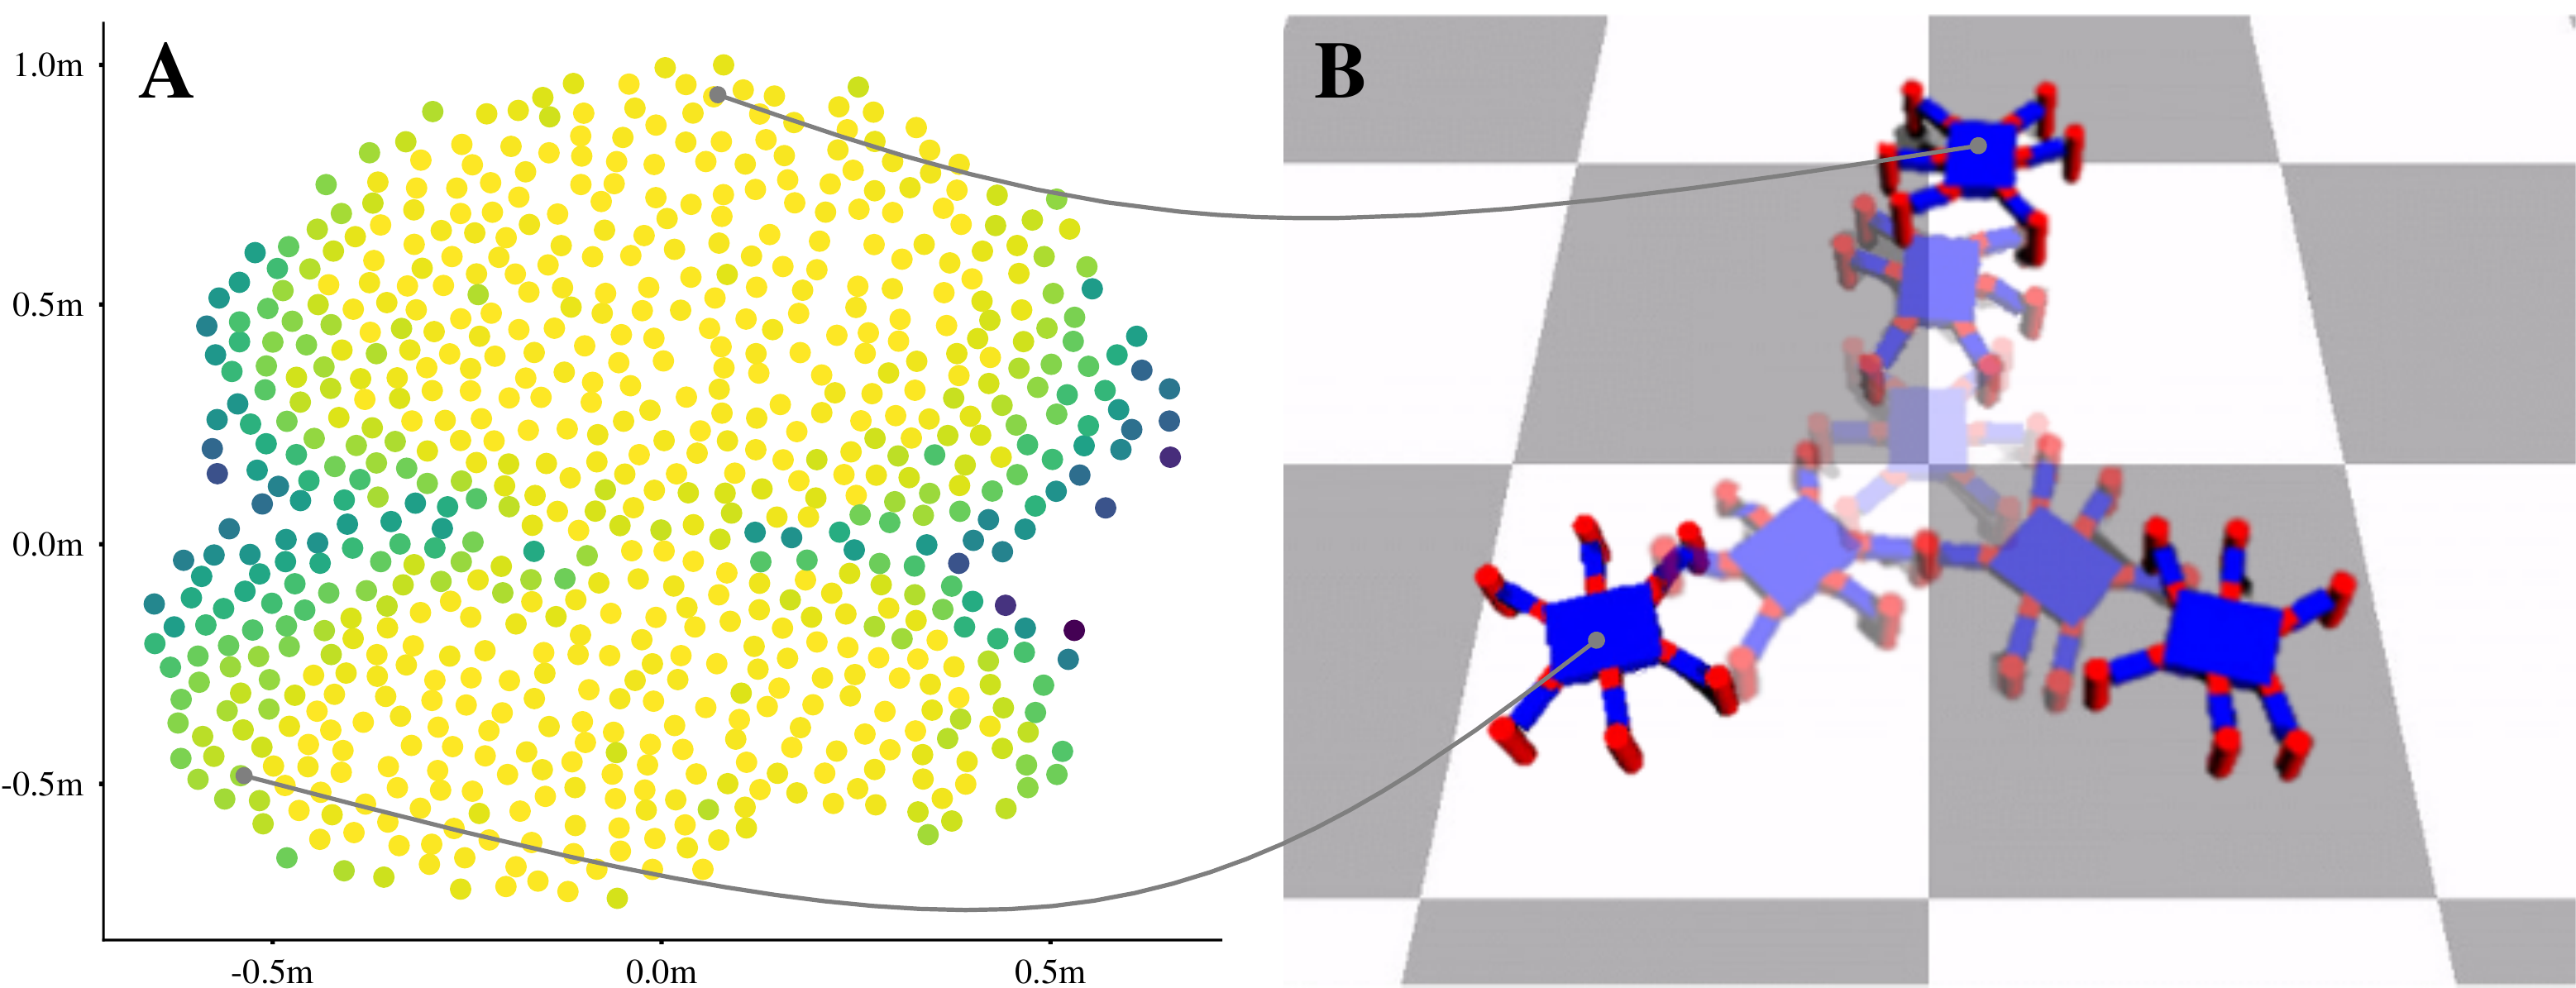}
\centering
\caption{
\textbf{Omni-directional Skill Repertoire.} 
(\textbf{A}) Skill repertoire learned by \algoname{} showing skills discovered with diverse final positions $\left(x_T,y_T\right)$. Each marker represents the skill descriptor of one policy; the color of each marker represents the return obtained by the policy. (\textbf{B}) \algoname{} discovers diverse locomotion skills; illustration of the execution of three sampled skills from the repertoire.
}\label{fig:omni-rep-viz}
\end{figure} 

\subsection{Hexapod Uni-directional Skill}
The new skill space referred to in section~\ref{sec:exps-continual} has the skill descriptor $\skilldescriptor$ defined as follows:
\begin{equation*}
    \skilldescriptor = 
    \begin{pmatrix}
    \frac{1}{K} \sum_k{U(\Theta_T(k) - 0.005 \pi)}  \\
    \frac{1}{K} \sum_k{U(-\Theta_T(k) - 0.005 \pi)}  \\ 
    \frac{1}{K} \sum_k{U(\Psi_T(k) - 0.005 \pi)}  \\
    \frac{1}{K} \sum_k{U(-\Psi_T(k) - 0.005 \pi)}  \\
    \frac{1}{K} \sum_k{U(\Phi_T(k) - 0.005 \pi)}  \\
    \frac{1}{K} \sum_k{U(-\Phi_T(k) - 0.005 \pi)}  \\
    \end{pmatrix}
\end{equation*}

where $U(\cdot)$ is the unit step function
$\Theta_T(k)$, $\Psi_T(k)$, and $\Phi_T(k)$ correspond respectively to the roll, pitch, and yaw angles of the robot's torso after an interval of $k=15\text{ms}$. $K$ represents the total number of 15ms intervals during an episode. The return $\reward$ is defined as:
\begin{equation*}
    \reward = x_T
\end{equation*}
where $x_T$ is the displacement in the forward direction at the end of the episode $T$.

This results in diverse ways of walking forward. This skill repertoire was taken from~\cite{cully2015robots} where it was used to show state-of-the-art damage recovery.

\subsection{Additional results for few-shot learning} \label{app:fewshot_ablation}
This section provides additional results for section \ref{sec:exps-zero_few_shot}. Table \ref{table:continual-ablation-results} shows extended results for the performance of the skills depending on the number of skills selected from the imagined repertoire when performing few-shot learning.

\begin{table*}[t]
\small
\centering
\begin{threeparttable}
\begin{tabular}{ lrrrr } 
 \toprule
 Algorithm & Evaluations & Best Return & Mean Return  & Repertoire Size \\
 \midrule 
 \algoname{} & $2{,}705\tnote{1}$ & $0.471$ & $0.191$ & $838$\\ 
%   \addlinespace
 Vanilla QD (Equivalent) & $3{,}000$ & $0.353$ & $0.068 $ & $662 $ \\
 Vanilla QD (Upper Baseline) & $100{,}000$ & $0.497$ & $0.177$ & $3{,}225$ \\ 
 %Vanilla QD (Equivalent) & $10{,}000$ & $0.41\pm0.027$ & $0.097\pm0.005$ & $1{,}320\pm 48$ \\
 %Vanilla QD (Equivalent) & $3{,}500$ & $0.37 \pm 0.04$ & $0.072 \pm 0.008$ & $744 \pm 28$ \\
 %\algoname{} (Direct Add) & $2,575 \pm 359$ & $0.47 \pm 0.07$ & $0.13 \pm 0.06$ & $2575 \pm 359$ \\ 
 \midrule
 \algoname{} (20-shot) & 20 & $0.33$ & $0.11$ & - \\ \algoname{} (15-shot) & 15 & $0.31$ & $0.11$ & - \\
 \algoname{} (10-shot) & 10 & $0.25$ & $0.11$ & - \\
 \algoname{} (5-shot) & 5 & $0.22$ & $0.10$ & -\\
 \algoname{} (2-shot) & 2 & $0.16$ & $0.11$ & -\\
 \algoname{} (Zero-shot) & 1 & $0.16$ & - & -\\ 
 \bottomrule
\end{tabular}
\end{threeparttable}
\vspace{2mm}
\caption{
Performance results obtained for \algoname{} in new skill acquisition, and for its equivalent and upper QD baselines.
The zero-shot and few-shot performance of \algoname{} are also displayed.
For each variant, we generated 10 different repertoires from independent replications and report the median.
%
%We report the medians of the results obtained from those replications.
\vspace{-8mm}
} \label{table:continual-ablation-results}
\end{table*}

\subsection{Reset-Free Trial and Error}
\label{appendix:rte-reset}
The skill repertoire $\archivereal$ returned by \algoname{} can be used to accomplish long-horizon tasks in the real world and also be leveraged for adaptation in the event of damage.
To do this, we use the Reset-free Trial and Error (RTE) algorithm \cite{chatzilygeroudis2018reset} based on the returned skill repertoires.
The RTE algorithm predicts the real-world outcomes of the skills from the repertoire, and uses those predicted outcomes as a basis for planning in the real-world environment.
RTE is divided into two phases (see Figure~\ref{fig:two_phase_qd}): the skill discovery phase (in simulation) and the planning phase.

During the skill discovery phase, a skill repertoire is learned via a QD algorithm, such as \algoname{} or MAP-Elites. The skill repertoire is then used as a prior for the Gaussian Processes.
Gaussian Processes (GPs) are then set to predict the difference between the outcomes in simulation and in the real world. 
Similarly to (Chatzilygeroudis et al., 2018) \cite{chatzilygeroudis2018reset}, we use GPs to learn the mapping: 
\begin{equation*}
    \left(\skilldescriptor \in \archivereal \right) \rightarrow \outcomegp_{real}
\end{equation*}
where $\outcomegp_{real}$ is a low-dimensional vector containing information about the robot displacement (such as the $(x, y)$ displacement, and the difference of orientation $\theta_{new} - \theta_{old}$).

During the planning phase, RTE uses these GP predictions together with a Monte-Carlo Tree Search (MCTS) planner to decide on the best action to execute.
After each executed action, the observed outcome $\outcomegp_{real}$ is measured and added to the GP datasets; the GP predictions are then updated accordingly. We then re-plan using these updated GP predictions at the next step.
The RTE algorithm keeps alternating between the MCTS planning and the GP updates until the task is solved. This re-planning along with online GP updates of the skill repertoire allows us to do online adaptation in the form of sim-to-real transfer and damage recovery, while performing a long-horizon task.

\begin{figure}[ht]
\centering
	\includegraphics[width=\linewidth]{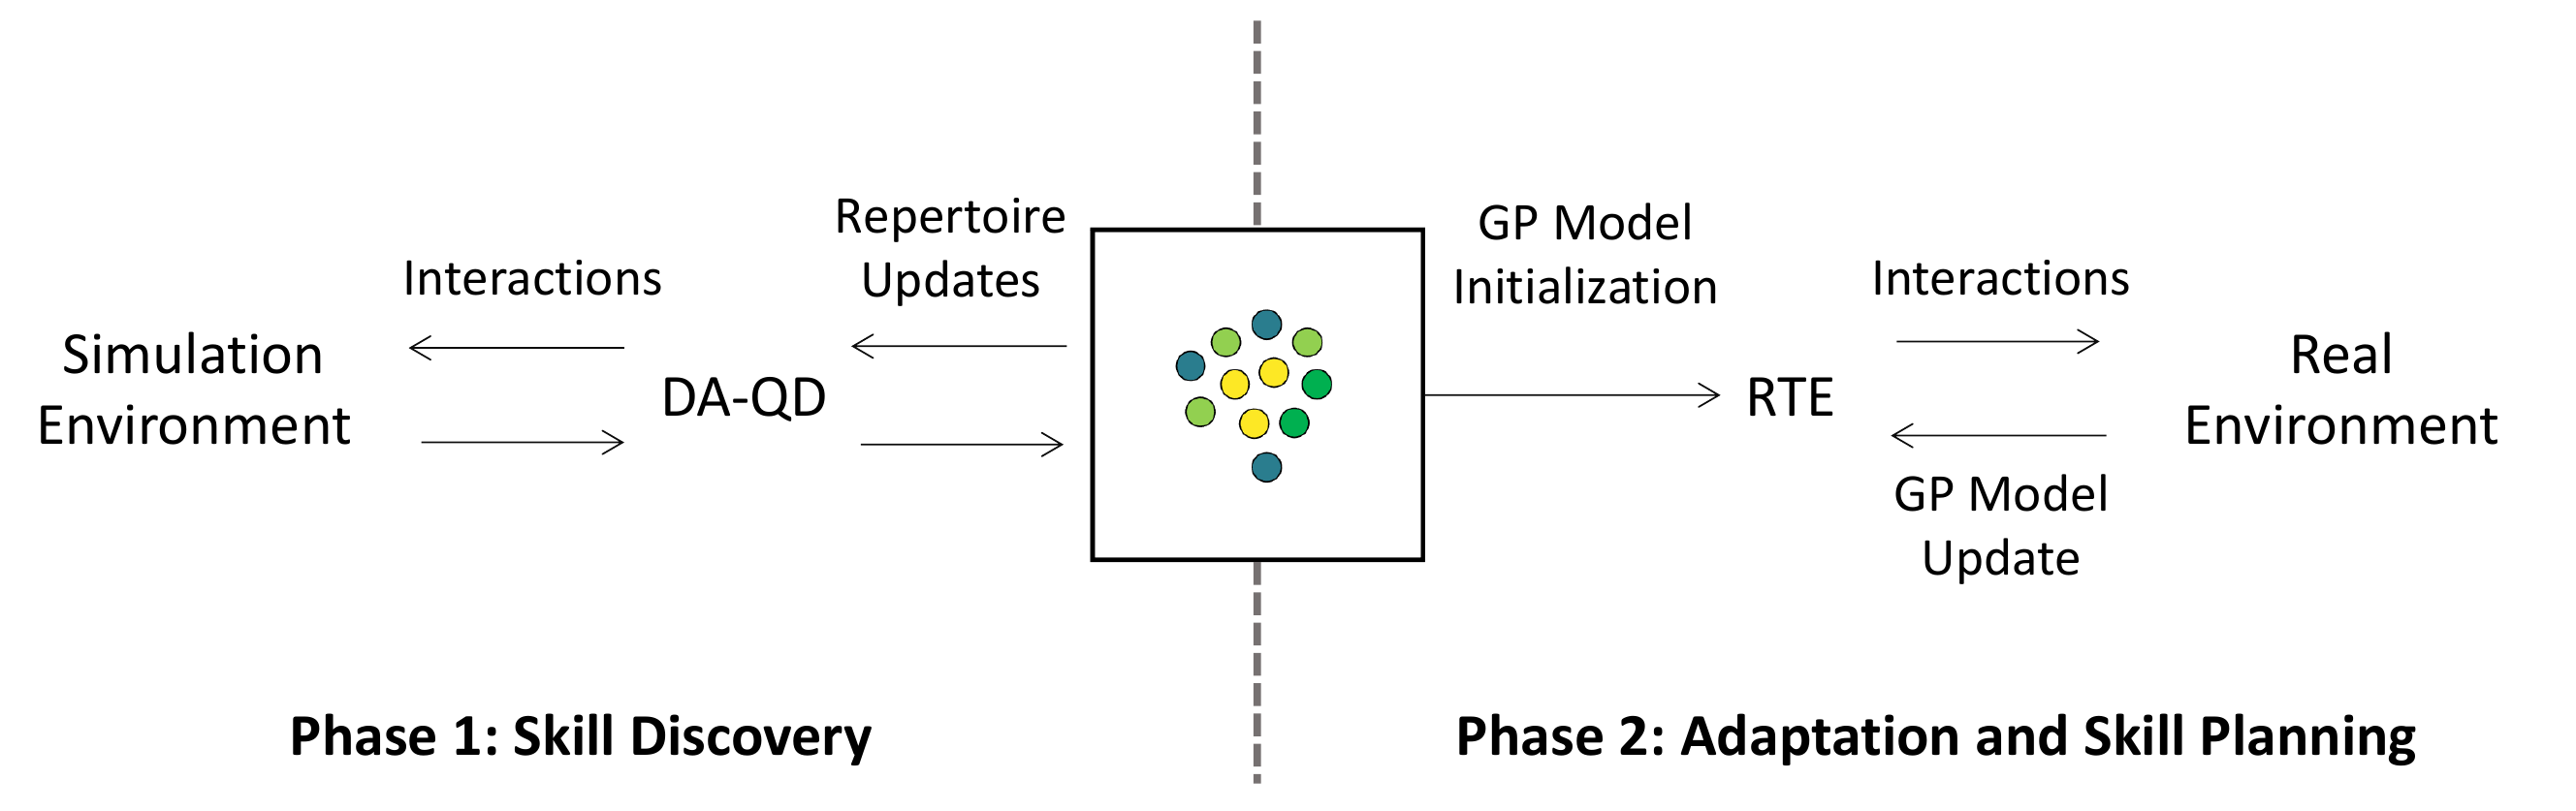}
\centering
\caption{
\textbf{Skill Discovery Phase}: Skills are discovered using any QD algorithm resulting in a repertoire of skills. \textbf{Planning Phase}: The skill repertoire produced is used by a planning algorithm to accomplish a long-horizon task. GP models which are used for rapid adaptation are also initialized with the skill repertoire.
}\label{fig:two_phase_qd}
\end{figure} 

\section{Quality-Diversity and other Skill Discovery Methods} \label{app:other-skill-discovery-methods}

% Bryan's option
Other methods for skill discovery in RL such as DIAYN~\cite{eysenbach2019diayn} and DADS~\cite{sharma2019dynamics} among others are based on Mutual Information (MI) maximization and different formulations of this MI objective. Quality-Diversity (QD) algorithms and MI maximization based algorithms have similar goals: \textbf{learning a repertoire of diverse policies} $\Pi$, where policies in this repertoire exhibit diverse behaviors.This objective can be summarized as maximizing the entropy of some function of the trajectories in this repertoire of policies.

\begin{align}
    \max H(f(\tau_i)) \pi_i \in \Pi
\end{align}

In both cases, the repertoire of policies can serve various purposes such as hierarchical planning~\cite{chatzilygeroudis2018reset, sharma2019dynamics} and adaptation to unforeseen situations~\cite{cully2015robots, chatzilygeroudis2018reset, kumar2020one}. The biggest difference between QD and MI maximization methods and where the methods diverge is the choice on how to represent the set of policies $\Pi$. QD algorithms opt to explicitly keep a population or repertoire (sometimes also referred to as an archive) of policies $\pi_i(a|s)$ while MI maximization methods represent these set of policies as a latent-conditioned policy $\pi(a|s,z)$. The difference in choice of representation arise due to how the methods function and how the policies are optimized.

Therefore, this section describes some of the similarities and differences between these methods.

\subsection{Differences}

\subsubsection{Problem Formulation}

As mentioned above, the difference in choice of the representation for the set of policies $\Pi$ are due to the underlying mechanisms of how these methods function. The representations matter as we want the diverse behaviors we obtain to be \textbf{controllable} by our policy. We have to somehow associate the policies in the repertoire to the diverse behaviors $f(\tau)$ we want as set in the objective.

\paragraph{QD Algorithms}

The QD family of algorithms, which originate from population-based methods~\cite{lehman2011evolving, pugh2016quality, cully2013behavioral, cully2017quality}, represents $\Pi$ explicitly as a repertoire of policies, keeping one policy $\pi_{\theta_i}$ for each skill. Each policy has an associated skill descriptor $\skilldescriptor_i$ which is obtained from rolling out the policy to obtain its trajectory $\tau_i$. The skill descriptor is just an encoding of this trajectory $\skilldescriptor_i = f(\tau_i)$. As explained in section \ref{sec:background}, new policies are only added to this repertoire $\Pi$ if they are novel (according to $\skilldescriptor$) or higher-performing. Maintaining this repertoire of policies is central to computing the novelty of policies and in driving the search towards more novel or higher-performing policies. As described in section \ref{sec:background}, the novelty is computed as the average Euclidean distance to its k-nearest neighbors in this repertoire. This novelty measure is used in the novelty search~\cite{lehman2011evolving} line of work but has recently been referred to also as particle-based entropy.
Controllability in this case is trivial because the parameters $\theta_i$ for each policy is explicitly kept as part of the repertoire $\Pi$ for each skill policy $\pi_{\theta_i}$.

%\begin{align}
%     = max H(f(\tau)) - H(f(\tau)|\pi_\theta)
%\end{align}

\paragraph{MI maximization algorithms}

MI maximization methods on the other hand represents the set of of policies $\Pi$ as a latent-conditioned policy $\pi(a|s,z)$. z is commonly sampled from an arbitrary uniform distribution before rolling out the policy. In this case, an additional term is added to the original objective to make the policy controllable by selecting a z, resulting in the MI maximization objective and its other formulations due to the symmetry of the MI.  

\begin{align}
     \max H(f(\tau)) - H(f(\tau)|z)
\end{align}

\begin{align}
     \max H(f(\tau)) - H(f(\tau)|z)
     = \max I(f(\tau), z)
     = \max H(z) - H(z|f(\tau)) 
\end{align}

As a result, MI maximization methods involve making an approximation for this intractable additional term in the form a variational lower bound. Learning this term is usually referred to as learning a discriminator $q(z|s)$ or skill dynamics $q(s_{t+1}|s_{t},z)$ depending on the MI formulation. The latent-conditioned policy is then optimized using off-the-shelf model-free RL algorithms which use these quantities as an intrinsic reward. 

Therefore, despite similar objectives, there is a fundamental difference in how diversity is driven in both methods arising from choice of policies. QD methods rely on maintaining a repertoire and novelty measures while MI maximization methods rely on learning a discriminator to separate the different behaviors along with model-free RL algorithms.
%biggest difference-> don't need a discriminator that is required to separate the different behaviors. Required for goal-conditioned policies. 

\subsubsection{Nature of Diversity}

%owever, even if the considered behavioral spaces are the same, 
The nature of behavioral characterizations between these methods are also different. 
The comparison here is akin to policy search based on evolutionary strategies and policy search based on gradient descent.

\paragraph{QD algorithms}

QD algorithms characterize their behaviors via skill descriptors. As introduced above, the skill descriptor is an encoding of the entire trajectory of a policy after being rolled-out $\skilldescriptor_i = f(\tau_{\pi_i})$.
QD maximizes the entropy (or spread) of the policies in the skill descriptor space.
In sections~\ref{sec:exps-sample_eff} and~\ref{sec:navigation}, the skill descriptors used for the hexapod correspond to the final $(x,y)$ position of each solution.
And in the zero-shot learning task (section~\ref{sec:exps-continual}), the skill descriptor for the new skill is a 6-dimensional vectors representing the average proportion of time the orientation of the robots torso is beyond an angular threshold value.
The return of the algorithm is a repertoire of different policies exhibiting behaviors that are diverse with respect to their skill descriptors.

\paragraph{MI maximization algorithms}

On the other hand, most MI maximization RL methods operate at the transition level.
It has been shown that maximizing the sum of MI between the states in the trajectory and $z$ lower bounds the MI between the entire trajectory and $z$: $I(\tau, z) \geq \sum_{t=1}^T I(s_t,z)$.
MI maximization RL considers an intrinsic reward designed to maximize the mutual information between the skill $\vec z$ and the states explored by the skill-conditioned policy $\pi \left( \cdot | \cdot, \vec z \right)$.
In the specific case of DADS, the purpose is to maximize the mutual information $I(\vec s_{t+1}, \vec z | \vec s_t)$ (mutual information between the robot's next state $\vec s_{t+1}$ and the skill $\vec z$, given the current state $\vec s_t$).
%
% The way it is implemented in DADS, when an $(x,y)$ prior is considered, the condition on the current $\vec s_t$ is removed, and the considered mutual information becomes $I(\Delta \vec s_t, \vec z)$.
%
The return of these algorithms is a single skill-conditioned policy, exhibiting diverse behaviors when sampling different skills $\vec z$.

\subsubsection{Gradient-based VS Gradient-free}

\paragraph{QD algorithms}

%As explained above, QD algorithms consider a single skill descriptor to characterize an entire trajectory.
%
%Hence, it is not straightforward to design a convenient reward function for optimizing a skill-conditioned policy using a off-the-shelf Reinforcement Learning (RL) algorithm which usually relies on transition level rewards.
%
Instead of relying on first-order optimization algorithms, QD algorithms generally rely on Evolutionary Algorithms or Evolutionary Strategies to drive the diversity during search.
Such techniques have the advantage of being easily parallelizable, usable with non-differentiable policies and controllers \cite{tang2020neuroevolution} and shown to be viable alternative for Reinforcement Learning \cite{salimans2017evolution}.
However, most of these algorithms suffer from a lack of sample efficiency, which is the motivation for our work in the context of QD algorithms.
Despite being gradient-free, there is nothing in the QD method that restricts using gradients. Recent work has shown impressive results when incorporating gradient-based methods into the QD framework~\cite{nilsson:hal-03135723} when neural network policies are used.
%
%And in the case of QD algorithms, the use of controllers with a high-number of parameters may affect negatively the performance of the algorithms.
%
%Several techniques have been explored to adapt QD optimization in the context of Deep Neuro-evolution (??); but such methods are are out of the scope of this paper.

\paragraph{MI maximization algorithms}

MI-based RL algorithms rely on deep RL algorithms to perform optimization of the policy. 
Hence, most components in these algorithms need to be differentiable and gradient based. 
As MI-based RL algorithms commonly operate at the transition level, they can define a trajectory-agnostic reward.
Maximizing the policy's return when considering this reward aims at maximizing the mutual information objective $I(\vec s_{t+1}, \vec z | \vec s_t)$ in the case of DADS.
Any RL algorithm with any gradient-based optimizer can be used to optimize the skill-conditioned policy.
Such gradient-based optimizers make it easy to train controllers having a large number of parameters such as neural networks.

\subsubsection{Task Reward}

\paragraph{QD algorithms}

QD algorithms inherently accommodate to task-related rewards. They prioritize the diversity of the learned policy repertoire, while locally maximizing the return of each policy.
For example, in the skill repertoire, a new solution is added to the repertoire if it is novel enough with respect to the solutions that are already present in it.
Then, each policy already present in the repertoire may be replaced by a policy having a better return and a similar skill descriptor (Local competition/optimization).

\paragraph{MI maximization algorithms}

DADS and DIAYN are exploration-only algorithms; as such, they rely exclusively on intrinsic task-agnostic rewards.
Recent work in MI-based RL such as SMERL~\cite{kumar2020one} have aimed to bring task-related reward into this line of work by formulating the problem as a Constrained Markov Decision Process (CMDP).
The CMDPs aim to maximize the diversity of a repertoire of policies, while also constraining the learned policies to achieve a minimal return on the task.
Solving those CMDPs leads to a repertoire of policies that are diverse among all the best-performing policies.

\subsection{Similarities}

%Quality-Diversity (QD) algorithms and Mutual-Information (MI) based algorithms attack the same problem: learning a collection of agents exhibiting diverse behaviors.
%
There is also some similarity between the ways behaviors are characterized among both these methods.
For example, most of the experiments performed in DADS~\cite{sharma2019dynamics} and DIAYN~\cite{eysenbach2019diayn} mention restricting the observation space to the x,y coordinates of the robot. The authors call this a \textit{prior}. Hence, the discriminator $q_{\vec \phi}$ (or skill-dynamics) used mostly rely on this $(x,y)$ \textit{prior}.
In that case, the discriminator $q_{\vec \phi}\left( \left(x,y\right)_{t+1} | \left(x,y\right)_{t}, \vec z \right)$ biases exploration towards diverse behaviors with respect to the $\left(x,y\right)$ space.

Similarly, this is analogous to Quality-Diversity algorithms which require the definition of a skill descriptor $\skilldescriptor$.
By defining the skill descriptor, we inject a prior over the dimensions and space where we want to see diversity.
In our locomotion experiments, the skill descriptors are similarly defined as the final $(x,y)$ coordinates of the robot which biases exploration towards diversity in the $(x,y)$ space.
Various types of skills descriptors can be used to characterize a behavior in the case of QD methods and defining it manually is just a way of injecting a prior on the diversity we desire.
However, in the case of where we do not have a prior or would like to learn a prior, there have been recent work to learn these skill descriptors in an unsupervised manner~\cite{cully2019autonomous, paolo2020unsupervised}. As mentioned in the main text, this is outside the scope of our contribution and we leave this for future work.

% \subsection{Learned Dynamics Components and Relationship to \algoname{}}

% Differences:
% \begin{itemize}
%     \item Method for achieving diverse skills -> lead to diverse behaviors but not diverse with respect to the same thing. DADS gets behaviors with different ways to go to different next states from the same current state. QD gets behaviors with diverse final positions (over the full trajectory).
%     \item Fitness.
%     \item Learned dynamics components. Can those be used for solving a new task?
%     \item gradient-based VS gradient free.
% \end{itemize}

% Why did we choose QD over DADS in the end?
% Why cannot we have a fair comparison between the two?

%\subsection{Relationship to our problem setting and why we do not use DADS}

\section{Quality-Diversity and Goal-Conditioned RL} \label{app:goal-conditioned-RL}
A recent study done by Choi et al.~\cite{choi2021variational} shows that Goal-Conditioned RL (GCRL) leads to a lower bound on the same objective as MI-maximization based methods and can be interpreted as a coarse variational approximation. GCRL can be interpreted as MI-maximization (or variational empowerment) algorihtm that has a fixed variational distribution. Conversely, skill-discovery via MI-maximization can be interpreted as a combination of representation learning and GCRL. They show that GCRL and prior-based variational empowerment (i.e. DIAYN) lie on different ends of the same spectrum. 

Hence, many of the points discussed above for QD and other skill discovery methods based on MI-maximization remain for Quality-Diversity and GCRL. The choice of representation for the set of policies remain as the main difference which arise from the different methodologies taken. There are also some documented similarities. Goal spaces in some cases and experimental setups can also be interpreted as the skill or behavior space in QD algorithms. QD algorithms can be seen as a population-based implementation of the well-known Intrinsically Motivated Goal Exploration Processes (IMGEP) framework as explained in Forestier et al.~\cite{forestier2017intrinsically}.

\clearpage
\pagenumbering{arabic}
\section*{Considerations for CoRL 2021 and the Pandemic} % add to a separate document or page - save it sepearately. 
Given social distancing restrictions and remote working orders caused by the pandemic, we had limited access to the lab and hardware to perform real-world experiments. We had hoped to do more real-world experiments to show how \algoname{} can be used directly in a real-world setting but had to focus on the final application of a resulting repertoire produced by \algoname{} in simulation due to the constraints on access. However, we still managed to conduct extensive real-world experiments in order to thoroughly evaluate our methodology. For all evaluations, we ensured enough replications were performed to assess the statistical significance. We also utilized open-sourced physics simulators which supplemented our real-world results while working remotely.

% we expected to do more - whihc is why we focused on the final aplication of the robot. 

% \section{Supplementary Experiments}
% \subsection{Validation of Dynamics Model}
% for Skill Descriptor and Return prediction

% \subsection{Addition Condition Ablations}
% In M-QD \cite{keller2020model}, they considered using threshold conditions for solutions evaluated by the surrogate model. $t_{nov}$ and $t_{qua}$. 

% % Explain or point to the paper section to explain how the threshold conditions work.

% The authors noted that the selection of these values of threshold were hyper-parameters that needed to be carefully chosen. Selecting threshold values that were too high would mean excessive confidence in the model's predictions and we prevent exploration of the skill space. On the other hand, selecting threshold values that were too low would allow most policies to be considered for evaluation and make the use of the model redundant.

% We first tried our experiments using similar threshold conditions. We used similar heuristics by selecting a $t_nov$ that was twice the distance of solutions in the archive and the same $t_qua$. We experimented with using the same archive addition conditions that were being used by the real archive. This gave us better results as shown in Figure \ref{}. We also found this to be much simpler as we do not need to tune the hyper-parameter values of $t_nov$ and $t_qua$ . However, these conditions are indeed more strict and are putting more confidence in the model's predictions.
